# Supplementary material for: Ensuring UAV Safety: A Vision-only and Real-time Framework for Collision Avoidance Through Object Detection, Tracking, and Distance Estimation
Source: arXiv:2405.06749 source file (2024-05-16)
Supplement: Supplementary file 1 [file appendix.tex]

\begin{table}[]
\centering
\begin{tabular}{|c|cccc|cccccc|}
\hline
\multirow{5}{*}{Model} & \multicolumn{4}{c|}{\multirow{4}{*}{Losses}}                                              & \multicolumn{6}{c|}{Metrics}                                                                                                                                                                                                                                                                                 \\ \cline{6-11} 
                       & \multicolumn{4}{c|}{}                                                                     & \multicolumn{2}{c|}{Regression}                                                        & \multicolumn{4}{c|}{Classification}                                                                                                                                                                                 \\ \cline{6-11} 
                       & \multicolumn{4}{c|}{}                                                                     & \multicolumn{1}{c|}{\multirow{3}{*}{RMSE}} & \multicolumn{1}{c|}{\multirow{3}{*}{MSE}} & \multicolumn{3}{c|}{Sliding Window}                                                                                                & \multirow{3}{*}{\begin{tabular}[c]{@{}c@{}}Accuracy \\ Threshold\end{tabular}} \\ \cline{8-10}
                       & \multicolumn{4}{c|}{}                                                                     & \multicolumn{1}{c|}{}                      & \multicolumn{1}{c|}{}                     & \multicolumn{1}{c|}{\multirow{2}{*}{Mean}} & \multicolumn{1}{c|}{\multirow{2}{*}{Max}} & \multicolumn{1}{c|}{\multirow{2}{*}{Min}} &                                                                                \\ \cline{2-5}
                       & \multicolumn{1}{c|}{Edge} & \multicolumn{1}{c|}{L1}   & \multicolumn{1}{c|}{Ssim} & Berhu & \multicolumn{1}{c|}{}                      & \multicolumn{1}{c|}{}                     & \multicolumn{1}{c|}{}                      & \multicolumn{1}{c|}{}                     & \multicolumn{1}{c|}{}                     &                                                                                \\ \hline
Unet                   & \multicolumn{1}{c|}{1.0}  & \multicolumn{1}{c|}{0.0}  & \multicolumn{1}{c|}{0.0}  & 0.0   & \multicolumn{1}{c|}{3.55}                  & \multicolumn{1}{c|}{3.39}                 & \multicolumn{1}{c|}{0.14}                  & \multicolumn{1}{c|}{0.14}                 & \multicolumn{1}{c|}{0.14}                 & 0.01                                                                           \\ \hline
Unet                   & \multicolumn{1}{c|}{0.0}  & \multicolumn{1}{c|}{1.0}  & \multicolumn{1}{c|}{0.0}  & 0.0   & \multicolumn{1}{c|}{0.43}                  & \multicolumn{1}{c|}{0.19}                 & \multicolumn{1}{c|}{0.61}                  & \multicolumn{1}{c|}{0.16}                 & \multicolumn{1}{c|}{0.71}                 & 0.86                                                                           \\ \hline
Unet                   & \multicolumn{1}{c|}{0.0}  & \multicolumn{1}{c|}{0.0}  & \multicolumn{1}{c|}{0.0}  & 1.0   & \multicolumn{1}{c|}{0.36}                  & \multicolumn{1}{c|}{0.12}                 & \multicolumn{1}{c|}{0.64}                  & \multicolumn{1}{c|}{0.17}                 & \multicolumn{1}{c|}{0.76}                 & 0.86                                                                           \\ \hline
Unet                   & \multicolumn{1}{c|}{0.0}  & \multicolumn{1}{c|}{0.5}  & \multicolumn{1}{c|}{0.0}  & 0.5   & \multicolumn{1}{c|}{0.37}                  & \multicolumn{1}{c|}{0.13}                 & \multicolumn{1}{c|}{0.66}                  & \multicolumn{1}{c|}{0.18}                 & \multicolumn{1}{c|}{0.74}                 & 0.89                                                                           \\ \hline
Unet                   & \multicolumn{1}{c|}{0.35} & \multicolumn{1}{c|}{0.25} & \multicolumn{1}{c|}{0.45} & 0.25  & \multicolumn{1}{c|}{0.39}                  & \multicolumn{1}{c|}{0.14}                 & \multicolumn{1}{c|}{0.63}                  & \multicolumn{1}{c|}{0.23}                 & \multicolumn{1}{c|}{0.72}                 & 0.86                                                                           \\ \hline
\end{tabular}
\caption{Accuracy \& Regression metrics for different losses}
\label{tab:result_table}
\end{table}
